# Supplementary material for: Monte Carlo simulations of vector pseudospins for strains: Microstructures, and martensitic conversion times
Source: arXiv:1506.07283 source file (2015-06-24)
Supplement: Supplementary file 1 [file Supplemental_Material.pdf]

**Supplementary Information for  
Monte Carlo simulations of vector pseudospins for strains: Microstructures, and  
martensitic conversion times**

N. Shankaraiah

*School of Physical Sciences, Jawaharlal Nehru University, New Delhi 110067, India.*

(Dated: June 24, 2015)

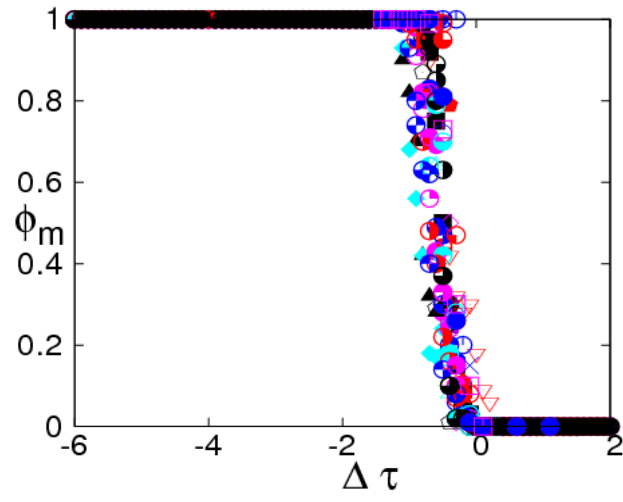

FIG. 1. *Conversion success-fraction for TCR, SO and TO transitions:* Plot of  $\phi_m$  versus  $\Delta\tau$  showing success fraction over 100 runs, for various  $A_1 = 1, 4, 10$ ,  $E_0 = 3, 4, 5, 6$  and fixed  $T_c/T_0 = 0.9$ .
